# Supplementary material for: Diffusion Denoised Smoothing for Certified and Adversarial Robust Out-Of-Distribution Detection
Source: arXiv:2303.14961 source file (2023-08-10)
Supplement: Supplementary file 2 [file settings.tex]

\section{Training, Datasets \& Resources}\label{app:settings}

In the context of DISTRO, we use the pre-trained diffusion model with 50M parameters, trained on \texttt{CIFAR10} with $1000$ steps and the cosine noise schedule~\citep{nichol2021improved}. 
Meanwhile, we trained the same model from scratch on \texttt{CIFAR100} for $1000$ steps, with a batch size of 128, a learning rate of 3$e$-4 and the cosine noise schedule.
The pretrained models OE, ATOM, ACET, ProoD and GOOD were trained with 80M Tiny Images~\cite{torralba200880} as OOD dataset.
The 80M Tiny Images dataset has been retracted because of concerns about offensive class labels. 
However, since previous studies have been conducted using this dataset, we compare our results to theirs.

We evaluate all methods on the standard datasets \texttt{CIFAR10/100}~\cite{cifar} as ID.
For the OOD detection evaluation we consider the following set of datasets: 
\texttt{CIFAR100/10}, \texttt{SVHN}~\cite{svhn}, LSUN~\cite{lsun} cropped (\texttt{LSUN\_CR}) and resized (\texttt{LSUN\_RS}) to $32\times32$,  TinyImageNet~\cite{tiny} cropped (\texttt{TinyImageNet\_CR}) to $32\times32$, \texttt{Textures}~\citep{textures} and synthetic (\texttt{Gaussian} and \texttt{Uniform}) noise distributions.
We use a random but fixed subset of 1000 images for all datasets considered as a test for OOD.
For ID, we consider the entire dataset.
We run all our experiments on a single NVIDIA A100.

\section{Adversarial AUC, AUPR and FPR}\label{app:adversarial}

Our goal is to maximize the confidence within the $\ell_\infty$-norm of adversarial attacks on OOD data.
We use an ensemble of projected gradient descent (PGD) \cite{madry2018towards} and 5000 queries with the black-box Square Attack \cite{squareattack}.
APGD \cite{apgd} is used with 500 iterations and 5 random restarts. The attack also includes a 200-step PGD with momentum of 0.9 and backtracking that starts with a step size of 0.1, which is halved if the gradient step does not increase confidence, and is multiplied by 1.1 otherwise.

Since robust OOD models are trained to be \textit{flat} on the out-distribution, disappearing gradients~\cite{pgd} pose a significant challenge for evaluating adversarial metrics~\cite{good, prood}.
As a result, a variety of starting points is necessary.
In following \citet{prood}, we start PGD from: 
i) a decontrasted version of the image, i.e. the point that minimizes the $\ell_\infty$-distance to the grey image $\{0.5\}^d$ within the threat model, ii) 3 uniform samples drawn from the threat model, and iii) 3 versions of the original image perturbed by Gaussian noise with $\sigma = 10^{-4}$ and then clipped to the threat model.
All steps of the attack are clipped to $[0,1]^d$, and the final score for OOD detection is directly optimized.
